# Supplementary material for: Magneto-transport properties of doped graphene
Source: arXiv:1907.08903 source file (2019-07-21)
Supplement: Supplementary file 1 [file Supplemental-Materials.pdf]

# Supplemental Materials

## Magneto-transport properties of doped graphene

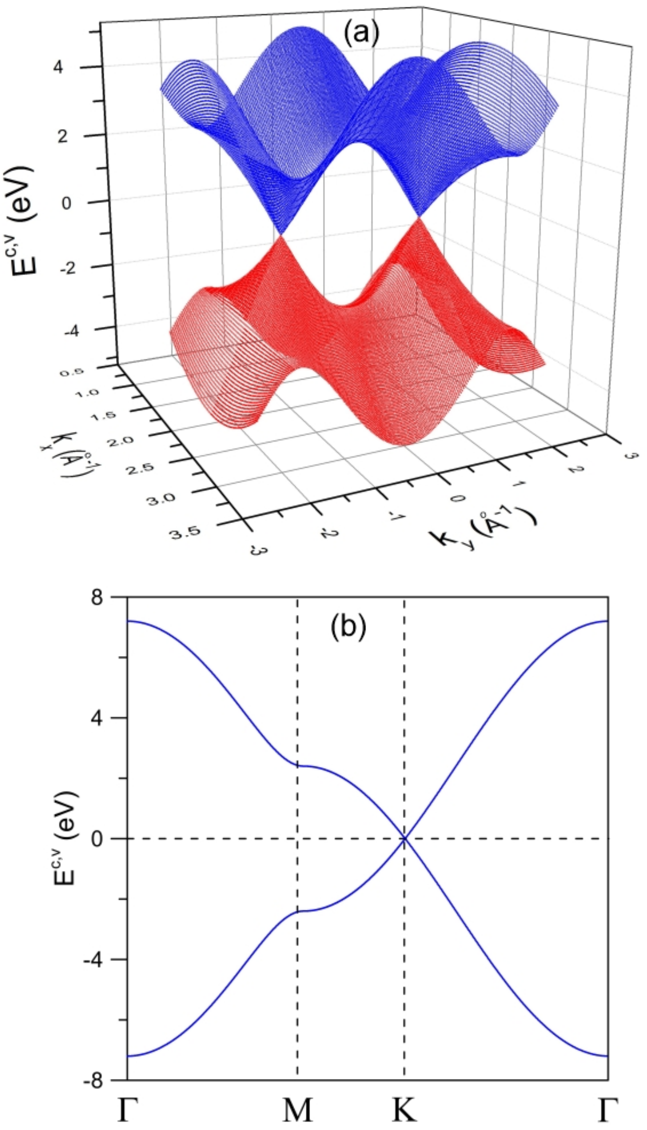


FIG. S1: (Color online) The (a) 3D energy band near the corner K and K′ points and (b) 2D energy bands of pristine graphene along high-symmetry points in the first Brillouin zone of Γ, M, and K. There exists a Dirac cone at each corner point with a Dirac point located right at zero energy. The occupied valence (red) and unoccupied conduction (blue) bands are symmetric about the Fermi level $E_F = 0$.

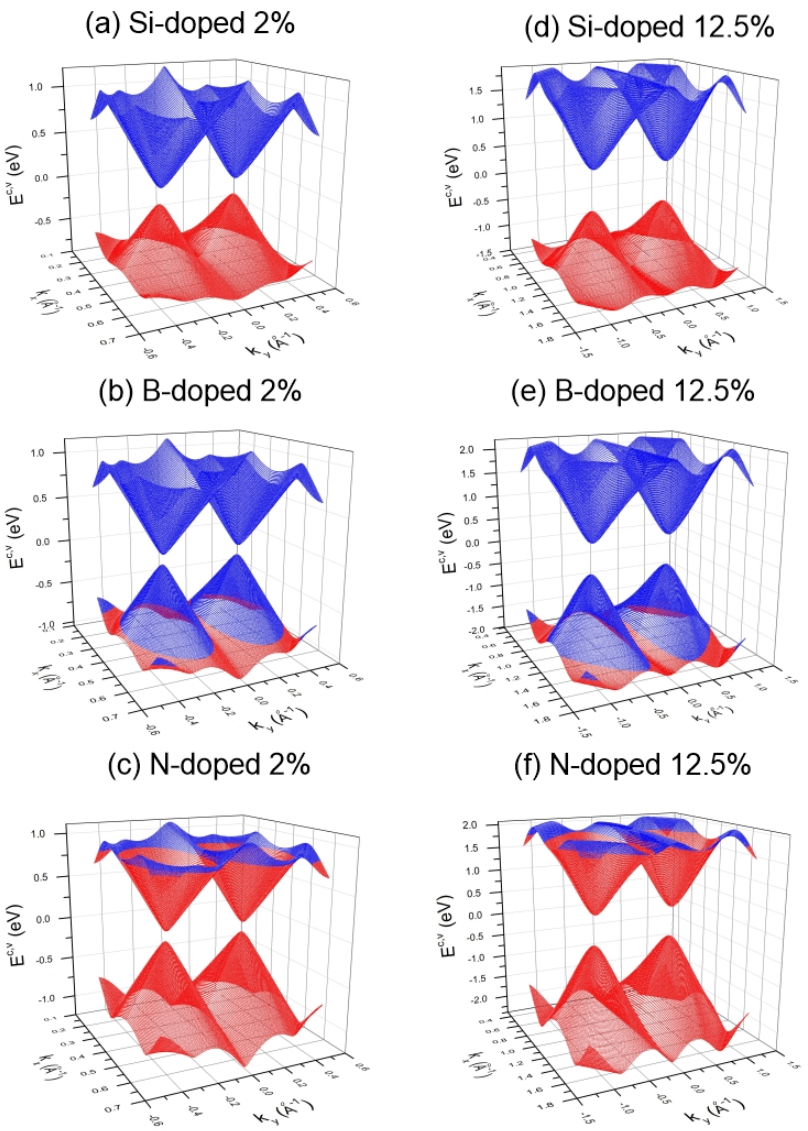


FIG. S2: (Color online) The 3D energy bands of doped graphene for Si, B, and N guest atoms with (a)-(c) 2% and (d)-(f) 12.5% concentrations, respectively. Doping opens a direct band gap near the zero energy with the size depending on the type and density of guest atoms. The Fermi energy remains the same for Si-doped, but shifts down for B-doped and shifts up for N-doped systems.

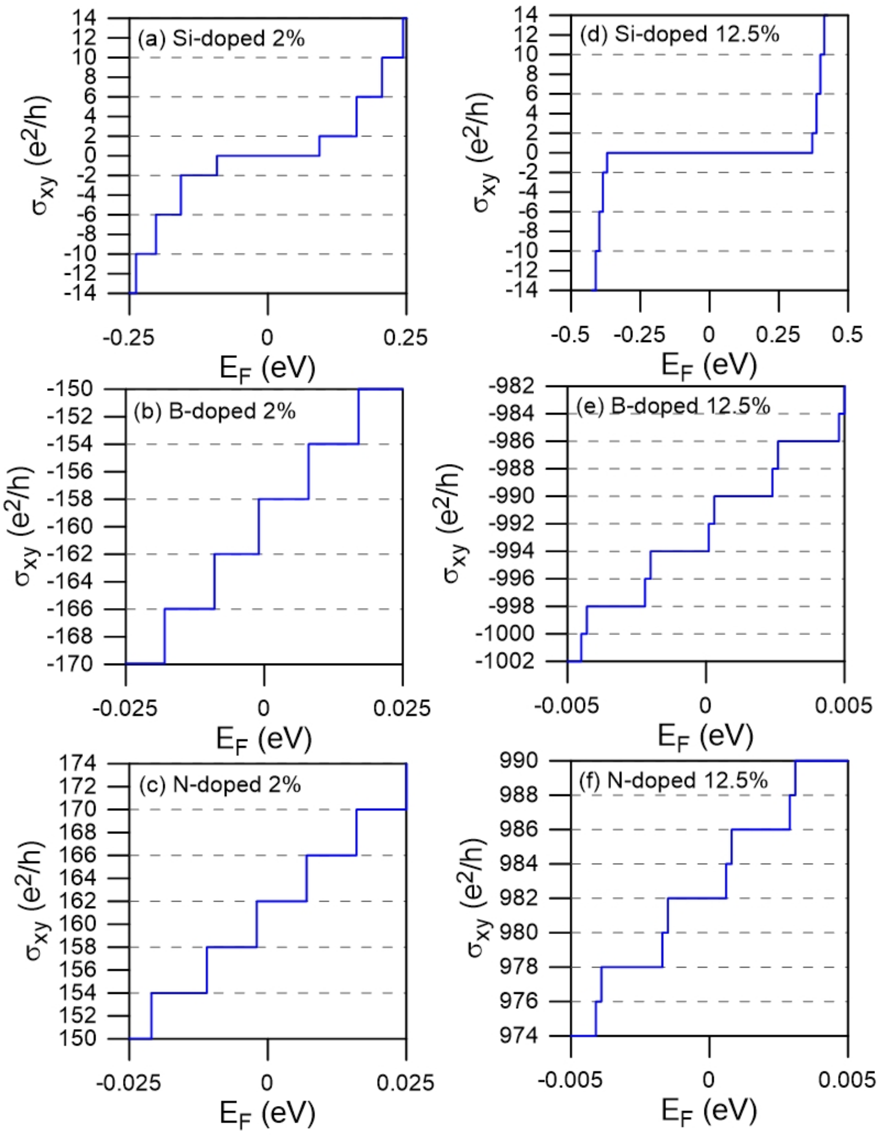


FIG. S3: (Color online) The $E_F$-dependent quantum Hall conductivity of Si-, B-, and N-doped graphene presents step structure, as demonstrated in (a)-(c) for 2% and (d)-(f) for 12.5% concentrations at $B_z = 20$ T . The emergence of zero conductivity, as shown in (a) and (d) for Si guest atom, is associated with the band gap created by the doping. The width of the plateau at zero energy, which directly reflects the size of the band gap, strongly depends on the dopants and doping concentrations. For B- and N-doped graphene, the split of LLs for 12.5% dopants are clearly reflected in the separation of the Hall plateaus, as illustrated in (e) and (f).
